# Supplementary material for: Intuitive joint priors for variance parameters
Source: arXiv:1902.00242 source file (2019-09-27)
Supplement: Supplementary file 1 [file tikzlibrarybayesnet.code.tex]

% tikzlibrary.code.tex
%
% Copyright 2010-2011 by Laura Dietz
% Copyright 2012 by Jaakko Luttinen
%
% This file may be distributed and/or modified
%
% 1. under the LaTeX Project Public License and/or
% 2. under the GNU General Public License.
%
% See the files LICENSE_LPPL and LICENSE_GPL for more details.

% Load other libraries
\usetikzlibrary{shapes}
\usetikzlibrary{fit}
\usetikzlibrary{chains}
\usetikzlibrary{arrows}

% Latent node
\tikzstyle{latent} = [circle,fill=white,draw=black,inner sep=1pt,
minimum size=20pt, font=\fontsize{10}{10}\selectfont, node distance=1]
% Observed node
\tikzstyle{obs} = [latent,fill=gray!25]
% Constant node
\tikzstyle{const} = [rectangle, inner sep=0pt, node distance=1]
% Factor node
\tikzstyle{factor} = [rectangle, fill=black,minimum size=5pt, inner
sep=0pt, node distance=0.4]
% Deterministic node
\tikzstyle{det} = [latent, diamond]

% Plate node
\tikzstyle{plate} = [draw, rectangle, rounded corners, fit=#1]
% Invisible wrapper node
\tikzstyle{wrap} = [inner sep=0pt, fit=#1]
% Gate
\tikzstyle{gate} = [draw, rectangle, dashed, fit=#1]

% Caption node
\tikzstyle{caption} = [font=\footnotesize, node distance=0] %
\tikzstyle{plate caption} = [caption, node distance=0, inner sep=0pt,
below left=5pt and 0pt of #1.south east] %
\tikzstyle{factor caption} = [caption] %
\tikzstyle{every label} += [caption] %

\tikzset{>={triangle 45}}

%\pgfdeclarelayer{b}
%\pgfdeclarelayer{f}
%\pgfsetlayers{b,main,f}

% \factoredge [options] {inputs} {factors} {outputs}
\newcommand{\factoredge}[4][]{ %
  % Connect all nodes #2 to all nodes #4 via all factors #3.
  \foreach \f in {#3} { %
    \foreach \x in {#2} { %
      \draw[-,#1] (\x) edge[-] (\f) ; %
    } ;
    \foreach \y in {#4} { %
      \draw[->,#1] (\f) -- (\y) ; %
    } ;
  } ;
}

% \edge [options] {inputs} {outputs}
\newcommand{\edge}[3][]{ %
  % Connect all nodes #2 to all nodes #3.
  \foreach \x in {#2} { %
    \foreach \y in {#3} { %
      \draw[->,#1] (\x) -- (\y) ;%
    } ;
  } ;
}

% \factor [options] {name} {caption} {inputs} {outputs}
\newcommand{\factor}[5][]{ %
  % Draw the factor node. Use alias to allow empty names.
  \node[factor, label={[name=#2-caption]#3}, name=#2, #1,
  alias=#2-alias] {} ; %
  % Connect all inputs to outputs via this factor
  \factoredge {#4} {#2-alias} {#5} ; %
}

% \plate [options] {name} {fitlist} {caption}
\newcommand{\plate}[4][]{ %
  \node[wrap=#3] (#2-wrap) {}; %
  \node[plate caption=#2-wrap] (#2-caption) {#4}; %
  \node[plate=(#2-wrap)(#2-caption), #1] (#2) {}; %
}

% \gate [options] {name} {fitlist} {inputs}
\newcommand{\gate}[4][]{ %
  \node[gate=#3, name=#2, #1, alias=#2-alias] {}; %
  \foreach \x in {#4} { %
    \draw [-*,thick] (\x) -- (#2-alias); %
  } ;%
}

% \vgate {name} {fitlist-left} {caption-left} {fitlist-right}
% {caption-right} {inputs}
\newcommand{\vgate}[6]{ %
  % Wrap the left and right parts
  \node[wrap=#2] (#1-left) {}; %
  \node[wrap=#4] (#1-right) {}; %
  % Draw the gate
  \node[gate=(#1-left)(#1-right)] (#1) {}; %
  % Add captions
  \node[caption, below left=of #1.north ] (#1-left-caption)
  {#3}; %
  \node[caption, below right=of #1.north ] (#1-right-caption)
  {#5}; %
  % Draw middle separation
  \draw [-, dashed] (#1.north) -- (#1.south); %
  % Draw inputs
  \foreach \x in {#6} { %
    \draw [-*,thick] (\x) -- (#1); %
  } ;%
}

% \hgate {name} {fitlist-top} {caption-top} {fitlist-bottom}
% {caption-bottom} {inputs}
\newcommand{\hgate}[6]{ %
  % Wrap the left and right parts
  \node[wrap=#2] (#1-top) {}; %
  \node[wrap=#4] (#1-bottom) {}; %
  % Draw the gate
  \node[gate=(#1-top)(#1-bottom)] (#1) {}; %
  % Add captions
  \node[caption, above right=of #1.west ] (#1-top-caption)
  {#3}; %
  \node[caption, below right=of #1.west ] (#1-bottom-caption)
  {#5}; %
  % Draw middle separation
  \draw [-, dashed] (#1.west) -- (#1.east); %
  % Draw inputs
  \foreach \x in {#6} { %
    \draw [-*,thick] (\x) -- (#1); %
  } ;%
}
